# Supplementary material for: From Silicon Shield to Carbon Lock-in ? The Environmental Footprint of Electronic Components Manufacturing in Taiwan (2015-2020)
Source: arXiv:2209.12523 source file (2022-09-26)
Supplement: Supplementary file 1 [file suppl-mat.pdf]

# Listing of electronic components manufacturers (ECMs) in Taiwan

| Company name | Fab location in Taiwan | CSR Data available | Taiwan-related data available | Within scope | Included in study | Specialization |
|---|---|---|---|---|---|---|
| **Included** | | | | | | |
| TSMC | Fab2, Fab3, Fab5, Fab12, Fab | Yes | Yes | Yes | Yes | Logic IC 5nm to 450nm; 6-inch to 12-inch |
| UMC | Fab6A, Fab8AB-N (Hsinchu) ; | Yes | Yes | Yes | Yes | 200nm IC / 300nm IC; 8-inch / 12-inch |
| Powerchip | FabP1, FabP2, FabP3, Fab8A | Yes | Yes | Yes | Yes | Power management IC / CMOS Image Sensor / Integrated Memory Chip / Discrete Devices for IGBT and Power MOS / LCD Driver IC (Opto) / SLC NAND Flash / Low Power DRAM; 12-inch |
| Vanguard | Fab1, Fab2 (Hsinchu) ; Fab3 (T | Yes | Yes | Yes | Yes | Display drivers IC / Power managemet IC / Discrete components; 8-inch |
| Global Wafers | Hsinchu | Yes | Yes | Yes | Yes | 3-inch to 12-inch silicon wafers |
| Nanya | Fab, Fab2 (Linkou) ; Fab3 (Nev | Yes | Yes | Yes | Yes | DRAM |
| Winbond | Memory Product Foundry (Taic | Yes | Yes | Yes | Yes | Flash Memory / Speciality DRAM / Mobile DRAM; 12-inch |
| Win Semiconductors | Fab A, Fab B, Fab C (Taoyuan) | Yes | Yes | Yes | Yes | GaAs devices |
| Epistar | FabF1 (Longtan) ; FabA1, N2, | Yes | Yes | Yes | Yes | LED (Opto) |
| Unimicron | Shanying, Luzhu, Hejiang, Zho | Yes | Yes | Yes | Yes | PCB / HDI / Carrier board / RF / IC Testing |
| Innolux | Zhunan, Tainan | Yes | Yes | Yes | Yes | TFT-LCD |
| Nuvoton | Hsinchu plant | Yes | Yes | Yes (partially) | Yes | General Purpose IC / Microcontrollers; 6-inch (Wafer mask manufacturing / testing / packaging) |
| Lextar | T01 (Hsinchu) | Yes | Yes | Yes | Yes | LED (Opto) |
| Everlight | Yuanli Plant, Shulin Plant, Tong | Yes | Yes | Yes | Yes | LED (Opto) |
| Optotech | Hsinchu | Yes | Yes | Yes | Yes | LED (Opto) |
| Wafer Works | Yangmei, Longtan | Yes | Yes | Yes | Yes | Wafer manufacturing |
| **Not included** | | | | | | |
| Siliconware Precision Industries | Dafong, Chungshan, Zhongke | Yes | Yes | No | No | IC packaging, processing, testing |
| Foxsemicon Integrated Technology | Hsinchu | Yes | No (not enough data) | – | No | – |
| Orient Semiconductor Electronics | Kaohsiung | Yes | No (not enough data) | – | No | – |
| Macronix | Fab2, Fab5, Fab1 (Hsinchu) | Yes | No (not enough data) | – | No | – |
| AUO | Fab L3D, L5D (Guishan) ; Fab | Yes | No | – | No | – |
| Global Foundries | USA, Germany, Singapore | Yes | No | – | No | – |
| Micron Memory Taiwan | Micron Memory (Taichung) / Fa | Yes | No | – | No | – |
| Merck Performance Materials | Kaohsiung | Yes | No | – | No | – |
| Panjit | Kaohsiung | Yes | No | – | No | – |
| Lite-On Semiconductor | Plant 1 (Keelung) / Plant 2 (Hsi | Yes | No | – | No | – |
| Delta Electronics | | Yes | No | – | No | – |
| Advanced Semiconductor Engineering Inc. (ASE Group +SPIL) | | Yes | No | – | No | – |
| Tatung Corp | | Yes | No | – | No | – |
| Acer | | Yes | No | – | No | – |
| Elan Microelectronics | Hsinchu, Zhonghe, Tainan, Kac | Yes | – | – | No | – |
| Formosa Sumco Technology | | Yes | – | – | No | – |
| Chipbond | Kuang-Fu, Li-Hsin Prosperity, F | Yes | – | – | No | – |
| Gudeng Precision | Tainan | No | – | – | No | – |
| Episil | Device Foundry, 6A, 6B (Hsinch | No | – | – | No | – |
| ProMOS | Fab4 (Taichung) | No | – | – | No | – |
| Taiwan Semi | Lije, I-Lan | No | – | – | No | – |
| Arima Optoelectronics | Hsinchu | No | – | – | No | – |
| AWSC | Tainan | No | – | – | No | – |
| SAN CHIH Semiconductor | Taoyuan | No | – | – | No | – |
| Creative Sensor Inc. | Wuxi Creative Sensor (Taipei) | No | – | – | No | – |
| Visera Technologies (Part of TSMC) | Headquarters Phase 1 (Hsinch | No | – | – | No | – |
| Episil | – | No | – | – | No | – |
| Creating Nano | – | No | – | – | No | – |
| Episil-Precision | – | No | – | – | No | – |
| Sun Yuan Technology | – | No | – | – | No | – |
| U-Can Dynatex | – | No | – | – | No | – |
| Ofuna Technology | – | No | – | – | No | – |
| Cin Phown Technology | – | No | – | – | No | – |
| Davicom Semiconductor | – | No | – | – | No | – |
| Holtek Semiconductor | – | No | – | – | No | – |
| Realtek Semiconductor | – | No | – | – | No | – |
| WiseChip Semiconductor | | No | – | – | No | – |
| Unikorn Semi | Hsinchu | No | – | – | No | – |
| Sigurd Microelectronics | Peishing, Chungshing, Hukou ( | No | – | – | No | – |
| Mosel Vitelic | | No | – | – | No | – |
| Kneron | | Not relevant | – | – | No | – |
| Green Energy Technology | | No | – | – | No | Solar panels |
| Sino-American Silicon Products | | No | – | – | No | Crystalline Wafer, Solar cell, Solar module |
| Hexawave | | No | – | – | No | – |
| **COUNT** | | **COUNT** | **COUNT** | **COUNT** | **COUNT** | |
| **60** | | **33** | **17** | **16** | **16** | |

*Notes* * The term "Electronic Components manufacturers" (ECM) can include: semiconductor manufacturing, passive eletronic component manufacturing, optoelectronic materials and components, other electronic component manufacturing.

*Sources*
https://www.tsia.org.tw/EN/MemberList?nodeID=59 (Criterion : Category « Manufacturing »)
https://www.semi.org/eu/resources/member-directory?search=&category%5B586%5D=586&country%5B681%5D=681&az (Criterion : Category « Semiconductor ; Semiconductor, Photonics » + Category « Device manufacturing » + Country «Taiwan»)
https://database.globalreporting.org/search/ (Criterion : Keyword « Semi » + Country «Taiwan»)
https://en.wikipedia.org/wiki/List_of_semiconductor_fabrication_plants (Criterion : Plant location «Taiwan»)

## Summary of results

| Year | 2015 | 2016 | 2017 | 2018 | 2019 | 2020 | CAGR |
|---|---|---|---|---|---|---|---|
| **GHG emissions (Unit : metric tons CO2e)** | | | | | | | |
| **THIS STUDY – GHG Emissions (Sc1+2)** | **13 085 218** | **14 158 264** | **15 712 523** | **16 969 309** | **17 200 259** | **18 770 908** | **7,5%** |
| Industry GHG emissions | 126 330 000 | 127 590 000 | 131 210 000 | 132 950 000 | 127 070 000 | ND | |
| THIS STUDY – share of Industry GHG emissions (%) | *10,4* | *11,1* | *12,0* | *12,8* | *13,5* | ND | |
| National GHG Emissions | 260 200 000 | 264 740 000 | 271 220 000 | 268 850 000 | 260 400 000 | ND | 0,0% |
| THIS STUDY – share of National GHG emissions (%) | *5,0* | *5,3* | *5,8* | *6,3* | *6,6* | ND | |
| THIS STUDY (SECTOR) - share of National GHG emissions (%) | *8,1* | *8,6* | *8,8* | *9,0* | *11,7* | ND | |
| **Final energy consumption (Unit : GWh)** | | | | | | | |
| **THIS STUDY – final energy consumption** | **18 947** | **20 495** | **25 131** | **26 515** | **27 904** | **31 403** | **8,8%** |
| Industry final energy consumption | 294 101 | 297 016 | 297 418 | 302 286 | 299 450 | 312 579 | 1,2% |
| THIS STUDY – share of Industry final energy consumption (%) | *6,4* | *6,9* | *8,4* | *8,8* | *9,3* | *10,0* | |
| National final energy consumption | 774 059 | 780 075 | 775 570 | 788 470 | 761 440 | 769 250 | -0,1% |
| THIS STUDY – share of national final energy consumption (%) | *2,4* | *2,6* | *3,2* | *3,4* | *3,7* | *4,1* | |
| THIS STUDY (SECTOR) - share of National final energy consumption (%) | *3,9* | *4,2* | *4,9* | *4,8* | *6,5* | *7,0* | |
| **Electricity consumption (Unit : GWh)** | | | | | | | |
| **THIS STUDY – electricity consumption** | **19 217** | **20 309** | **22 807** | **25 131** | **26 505** | **29 421** | **8,9%** |
| Industry electricity consumption | 134 700 | 136 890 | 141 111 | 148 961 | 147 675 | 150 742 | 2,3% |
| THIS STUDY – share of Industry electricity consumption (%) | *14,3* | *14,8* | *16,2* | *16,9* | *17,9* | *19,5* | |
| National electricity consumption | 250 019 | 255 420 | 261 394 | 266 568 | 265 720 | 271 247 | 1,6% |
| THIS STUDY – share of national electricity consumption (%) | *7,7* | *8,0* | *8,7* | *9,4* | *10,0* | *10,8* | |
| THIS STUDY (SECTOR) - share of National electricity consumption (%) | *12,3* | *12,8* | *13,3* | *13,4* | *17,7* | *18,7* | |
| **Water consumption (Unit : m3)** | | | | | | | |
| **THIS STUDY – water consumption** | **107 207 300** | **105 927 409** | **117 015 590** | **123 979 533** | **129 511 532** | **144 040 335** | **6,1%** |
| Industry water consumption | 1 601 000 000 | 1 629 000 000 | 1 654 000 000 | 1 668 000 000 | 1 671 350 000 | 1 803 190 000 | 2,4% |
| THIS STUDY – share of Industry water consumption (%) | *6,7* | *6,5* | *7,1* | *7,4* | *7,7* | *8,0* | |
| National water consumption | 16 025 000 000 | 16 546 000 000 | 16 645 000 000 | 16 713 000 000 | 16 739 280 000 | 16 675 930 000 | 0,8% |
| THIS STUDY – share of National water consumption (%) | *0,7* | *0,6* | *0,7* | *0,7* | *0,8* | *0,9* | |

## Indexes of environmental impacts and manufacture of electronic parts and components

| 2016=100 | 2015 | 2016 | 2017 | 2018 | 2019 | 2020 | CAGR |
|---|---|---|---|---|---|---|---|
| THIS STUDY – GHG Emissions (Sc1+2) | 92,4 | 100,0 | 111,0 | 119,9 | 121,5 | 132,6 | 7,48% |
| THIS STUDY – Electricity consumption | 94,6 | 100,0 | 112,3 | 123,7 | 130,5 | 144,9 | 8,89% |
| THIS STUDY – Water consumption | 101,2 | 100,0 | 110,5 | 117,0 | 122,3 | 136,0 | 6,08% |
| Manufacture of Integrated Circuits | 88,1 | 100,0 | 109,4 | 119,0 | 120,7 | 153,9 | 11,80% |

## Study representativeness of Taiwanase ECM industry

| Year | 2015 | 2016 | 2017 | 2018 | 2019 | 2020 | (min) | (max) | (average) |
|---|---|---|---|---|---|---|---|---|---|
| Autoproducers share of national electricity generation | 16,40 | 16,44 | 16,17 | 15,22 | 15,53 | 16,00 | | | |
| Independent power producers share of national electricity generation | 15,55 | 14,97 | 14,37 | 15,81 | 15,93 | 15,78 | | | |
| Taipower share of national electricity generation | 68,05 | 68,59 | 69,46 | 68,97 | 68,54 | 68,22 | | | |
| Share of Taipower ECM electricity consumption | ND | 62,34 | 65,82 | 70,23 | 56,31 | 57,94 | | | |
| **Representativness of study based on Taipower data** | **ND** | **62,3** | **65,8** | **70,2** | **56,3** | **57,9** | 56 | 70 | 62,5 |

*Sources*

MOEA, Energy Statistics Handbook 2020 p.83-84 ; Taipower Open Data, 台灣電力公司_
歷年售電量(用途別) (https://data.gov.tw/dataset/35392)

https://www.moeaboe.gov.tw/ECW/main/content/wHandMenuFile.ashx?file_id=1411

https://www.moeaboe.gov.tw/ECW/english/content/ContentLink.aspx?menu_id=1540

Taipower produces about 70% of the electricity on the island but it is the main electricity vendor for ECMs. We therefore consider Taiwpower's electricity to represent 100% of the sub-sector.

# Final energy and electricity consumption of selected electronic components manufacturers

| *Unit : GWh* | Final energy consumption | | | | | | | | Electricity consumption | | | | | | | | |
|---|---|---|---|---|---|---|---|---|---|---|---|---|---|---|---|---|---|
| **Year** | **2015** | **2016** | **2017** | **2018** | **2019** | **2020** | ***Diff 2015/2020 (%)*** | | **2015** | **2016** | **2017** | **2018** | **2019** | **2020** | ***Diff 2015/2020 (%)*** | *Notes* | *Sources* |
| TSMC | 8 915 | 9 848 | 12 016 | 13 167 | 14 327 | 16 900 | *90* | Electricity consumption represents 94% of final energy consumption (2018-2020) | 8 460 | 9 358 | 11 388 | 12 441 | 13 580 | 16 030 | *89* | *910 GWh of Renewable Energy, R* | *TSMC CSR Report 2019-2021* |
| Innolux | 5 092 | 4 906 | 5 251 | 5 259 | 5 388 | 5 857 | *15* | | 4 955 | 4 774 | 5 109 | 5 117 | 5 243 | 5 263 | *6* | | *Innolux CSR Report 2019-2020* |
| Unimicron | 853 | 860 | 947 | 1 028 | 1 059 | 1 107 | *30* | | 780 | 785 | 873 | 940 | 975 | 1 023 | *31* | | *Unimicron CSR Report 2019-2020* |
| UMC | 2 538 | 2 512 | 2 748 | 2 738 | 2 728 | 2 780 | *10* | | 2 306 | 2 290 | 2 542 | 2 534 | 2 534 | 2 581 | *12* | | *UMC CSR Report 2019-2020* |
| Powerchip | ND* | ND* | 1 171 | 1 178 | 1 232 | 1 267 | | | 803 | 811 | ND* | 1 062 | 1 102 | 1 135 | *41* | | *Powerchip CSR Report 2019-2020* |
| Vanguard | 705 | 713 | 709 | 714 | 695 | 882 | *25* | | 665 | 669 | 666 | 676 | 667 | 855 | *29* | | *Vanguard CSR Report 2019-2020* |
| Global Wafers | ND | ND | 367 | 362 | 325 | 328 | | | ND | ND | 367 | 362 | 325 | 328 | *ND* | | *GlobalWafers CSR Report 2019-2020* |
| Nanya | ND | 454 | 615 | 689 | 757 | 759 | | | 402 | 430 | 576 | 645 | 709 | 712 | *77* | | *Nanya CSR Report 2015-2016-2019-2020* |
| Winbond | 429 | 442 | 510 | 562 | 589 | 613 | *43* | | 380 | 390 | 453 | 498 | 528 | 546 | *44* | | *Winbond CSR Report 2017-2018-2020* |
| Epistar | ND* | 332 | 318 | 322 | 315 | 305 | | | ND* | 321 | 305 | 308 | 299 | 290 | *ND* | | *Epistar CSR Report 2018-2020* |
| Win Semiconductors | 79 | 80 | 121 | 138 | 147 | 167 | *111* | | 73 | 75 | 113 | 128 | 138 | 158 | *116* | | *Win CSR Report 2018-2019-2020* |
| Nuvoton | 80 | 80 | 78 | 77 | 76 | 75 | *-6* | | 78 | 77 | 75 | 74 | 73 | 72 | *-8* | | *Nuvoton CSR Report 2019-2020* |
| Lextar | 100 | 96 | 92 | 89 | 77 | 71 | *-29* | | 100 | 96 | 92 | 88 | 77 | 71 | *-29* | | *Lextar CSR Report 2016-2017-2018-2020* |
| Everlight | 44 | 51 | 66 | 63 | 63 | 165 | *275* | | 44 | 51 | 65 | 62 | 62 | 163 | *270* | | *Everlight CSR Report 2019-2020* |
| Optotech | ND | ND | ND | ND | ND | ND | | | 64 | 67 | 66 | 72 | 72 | 72 | *13* | | *Optotech CSR Report 2017-2019* |
| Wafer Works | 112 | 121 | 123 | 130 | 127 | 128 | *14* | | 107 | 115 | 117 | 124 | 121 | 122 | *14* | | *Wafer Works CSR Report 2016-2018-2020* |
| **Subtotal** | **18 947** | **20 495** | **25 131** | **26 515** | **27 904** | **31 403** | *66* | | **19 217** | **20 309** | **22 807** | **25 131** | **26 505** | **29 421** | *53* | | |
| All ECM except TSMC | 10 032 | 10 647 | 13 115 | 13 348 | 13 577 | 14 503 | *45* | All ECM except TSMC | 10 757 | 10 951 | 11 419 | 12 690 | 12 925 | 13 391 | *24* | | |

ND = No Data

(*) : CSR department contacted but didn't answer

Electricity comsumption is reported more often than final energy which explains why final energy reported is lower or equal to electricity consumption in 2015 and 2016

# Taiwan national energy consumption

| *Unit : GWh* | | | | | | | | | |
|---|---|---|---|---|---|---|---|---|---|
| **Year** | **2015** | **2016** | **2017** | **2018** | **2019** | **2020** | ***Diff 2015/2020 (%)*** | **Source** | **Notes** |
| **Final energy consumption** | | | | | | | | | |
| National final energy consumption | 774 059 | 780 075 | 775 570 | 788 470 | 761 440 | 769 250 | *-1* | MOEA, Energy Statistics | Handbook 2020 ; https://eng.stat.gov.tw/ct.asp?xItem=18741&CtNode=4942&mp=5 |
| Industry final energy consumption | 294 101 | 297 016 | 297 418 | 302 286 | 299 450 | 312 579 | *6* | | |
| Industry share of final energy use | 38,0 | 38,1 | 38,3 | 38,3 | 39,3 | 40,6 | | | |
| **Electricity consumption** | | | | | | | | | |
| National electricity consumption | 250 019 | 255 420 | 261 394 | 266 568 | 265 720 | 271 247 | *8* | | |
| Industry electricity consumption | 134 700 | 136 890 | 141 111 | 148 961 | 147 675 | 150 742 | *12* | | |
| Industry share of national electricity consumption | 53,9 | 53,6 | 54,0 | 55,9 | 55,6 | 55,6 | | | |
| **Taipower data** | | | | | | | | | |
| ECM electricity consumption reported by Taipower | ND | 32 579 | 34 649 | 35 782 | 47 070 | 50 780 | | Taipower Open Data, 台 | Dataset perimeter changed in 2019, hence the reported consumption gets bigger |
| Share of ECM electricity consumption reported by Ta | ND | 23,8 | 24,6 | 24,0 | 31,9 | 33,7 | | | |
| **Study scope** | | | | | | | | | |
| **THIS STUDY – Final energy consumption of sele** | **18 947** | **20 495** | **25 131** | **26 515** | **27 904** | **31 403** | ***65,7*** | | |
| Share of industry final energy consumption | 6,4 | 6,9 | 8,4 | 8,8 | 9,3 | 10,0 | | | |
| **THIS STUDY – Electricity consumption of selecte** | **19 217** | **20 309** | **22 807** | **25 131** | **26 505** | **29 421** | ***53,1*** | | |
| Share of Industry electricity consumption | 14,3 | 14,8 | 16,2 | 16,9 | 17,9 | 19,5 | | | |
| Share of national electricity consumption | 7,7 | 8,0 | 8,7 | 9,4 | 10,0 | 10,8 | | | |
| Share of Taipower ECM electricity consumption | ND | 62,3 | 65,8 | 70,2 | 56,3 | 57,9 | | | Min [%]: 56,3 \| Max [%]: 70,2 |
| Share of electricity in final energy consumption | 101,43% | 99,10% | 90,75% | 94,78% | 94,98% | 93,69% | | | Average [%]: 94,5 |
| **Other sectors** | | | | | | | | | |
| Agriculture electricity consumption | 2 917 | 2 922 | 3 037 | 2 960 | 3 045 | 3 273 | *12* | | |
| Transport electricity consumption | 1 391 | 1 402 | 1 463 | 1 469 | 1 499 | 1 481 | *6* | | |
| Services electricity consumption | 47 137 | 47 957 | 48 317 | 47 119 | 46 736 | 46 237 | *-2* | | |
| Residential electricity consumption | 44 882 | 47 332 | 47 612 | 46 879 | 47 189 | 50 207 | *12* | | |
| Industry electricity consumption | 134 700 | 136 890 | 141 111 | 148 961 | 147 675 | 150 742 | *12* | | |
| Energy electricity consumption | 18 990 | 18 914 | 19 852 | 19 178 | 19 574 | 19 306 | *2* | | |

# Conversion tables

| **Year** | **2015** | **2016** | **2017** | **2018** | **2019** | **2020** | | |
|---|---|---|---|---|---|---|---|---|
| **Umimicron (as reported)** | | | | | | | Notes | |
| Natural gas (m3) | 5 690 240 | 6 147 126 | 6 005 930 | 7 531 420 | 7 881 489 | 7 780 200 | Conversion factor (m3 to MWh) | |
| Conversion MWh | 60 032 | 64 852 | 63 363 | 79 456 | 83 150 | 82 081 | | 0,01055 |
| Fuel oil (Liter) | 422 000 | 450 000 | 488 000 | 512 000 | 0 | 0 | Conversion factor | |
| Conversion MWh | 4 937 | 5 265 | 5 710 | 5 990 | 0 | 0 | | 0,0117 |
| Diesel fuel (Liter) | 724 000 | 450 000 | 411 000 | 182 000 | 77 000 | 128 000 | Conversion factor (diesel liter to MWh) | |
| Conversion MWh | 7 776 | 4 833 | 4 414 | 1 955 | 827 | 1 375 | | 0,01074 |
| Gasoline (Liter) | 5 000 | 9 000 | 13 000 | 15 000 | 11 000 | 11 000 | Conversion factor (gasoline liter to MWh) | |
| Conversion MWh | 45 | 80 | 116 | 134 | 98 | 98 | | 0,0089 |
| Electricity consumption (MWh) | 780 000 | 785 000 | 873 000 | 940 000 | 975 000 | 1 023 000 | | |
| **TOTAL (final energy)** | **852 790** | **860 030** | **946 602** | **1 027 535** | **1 059 075** | **1 106 554** | | |
| **Nanya (as reported)** | | | | | | | | |
| Electricity consumption (MWh) | ND | 430 000 | 576 000 | 645 000 | 709 000 | 712 000 | | |
| Natural gas consumption (MWh) | ND | 23 818 | 38 092 | 44 151 | 47 545 | 46 743 | | |
| Diesel fuel (Liter) | ND | ND | 70 000 | 14 400 | 20 000 | 17 720 | Conversion factor (diesel liter to MWh) | |
| Conversion MWh | ND | ND | 752 | 155 | 215 | 190 | | 0,01074 |
| **TOTAL (final energy)** | | **453 818** | **614 844** | **689 306** | **756 760** | **758 933** | | |
| **Epistar (as reported)** | | | | | | | | |
| Diesel fuel (GJ) | 270 | 390 | 344 | 411 | 7 442 | 427 | Conversion factor (GJ to MWh) | |
| Conversion MWh | 75 | 108 | 96 | 114 | 2 067 | 119 | | 0,2778 |
| Natural gas (GJ) | 50 570 | 38 860 | 46 192 | 49 290 | 49 120 | 53 103 | Conversion factor (GJ to MWh) | |
| Conversion MWh | 14 048 | 10 795 | 12 832 | 13 693 | 13 646 | 14 752 | | 0,2778 |
| Electricity consumption (MWh) | ND | 321 000 | 305 000 | 308 000 | 299 000 | 290 000 | | |
| **TOTAL (final energy)** | | **331 904** | **317 928** | **321 807** | **314 713** | **304 871** | | |
| **Siliconware Precision Industries (as reported)** | | | | | | | | |
| Natural gas consumption (MJ) | 26 341 397 | 41 244 081 | 46 869 437 | 47 800 848 | 54 725 702 | ND | Conversion MJ to MWh | |
| Conversion MWh | 7 318 | 11 458 | 13 020 | 13 279 | 15 203 | - | | 0,0002778 |
| Electricity consumption (MWh) | 106 712 | 115 345 | 116 720 | 123 832 | 120 943 | 121 886 | | |
| **TOTAL (final energy)** | **114 030** | **126 803** | **129 740** | **137 111** | **136 146** | **1 266 000** | | |
| **Wafer Works** | | | | | | | | |
| Power (MJ) | 384 132 226 | 415 208 416 | 420 158 369 | 445 760 640 | 435 360 452 | 438 753 812 | Conversion MJ to MWh | |
| Conversion MWh | 106 712 | 115 345 | 116 720 | 123 832 | 120 943 | 121 886 | | 0,0002778 |
| Conversion electricity consumption (MWh) | 106 712 | 115 345 | 116 720 | 123 832 | 120 943 | 121 886 | | |
| Diesel (MJ) | 955 273 | 745 530 | 542 800 | 391 469 | 271 064 | 322 927 | Conversion MJ to MWh | |
| Conversion MWh | 265 | 207 | 151 | 109 | 75 | 90 | | 0,0002778 |
| Natural Gas (MJ) | 18 685 666 | 19 866 883 | 20 945 187 | 20 912 771 | 21 342 975 | 21 236 076 | Conversion MJ to MWh | |
| Conversion MWh | 5 191 | 5 519 | 5 819 | 5 810 | 5 929 | 5 899 | | 0,0002778 |
| **TOTAL (final energy)** | **111 903** | **120 864** | **122 539** | **129 642** | **126 872** | **127 785** | | |

# Energy mix in Taiwan

| **Year** | **2015** | **2016** | **2017** | **2018** | **2019** | **2020** |
|---|---|---|---|---|---|---|
| Coal | - | - | - | - | - | 45,3 |
| Gas | - | - | - | - | - | 36,0 |
| Oil | - | - | - | - | - | 1,5 |
| Nuclear | - | - | - | - | - | 11,2 |
| All renewables | - | - | - | - | - | 5,9 |
| Hydro | - | - | - | - | - | 2,2 |
| Solar | - | - | - | - | - | 2,2 |
| Wind | - | - | - | - | - | 0,9 |
| Other renewables including bioenergy | - | - | - | - | - | 0,7 |

Source : https://www.iea.org/countries/chinese-taipei

Source : https://ourworldindata.org/energy/country/taiwan

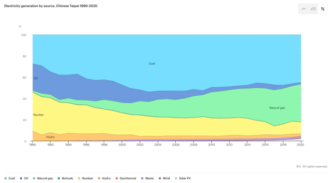


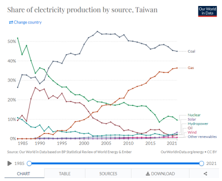

# Greenhouse Gases Emissions of selected electronic components manufacturers

| *Unit : metric tons CO2e* | Greenhouse Gases Emissions (Scope 1) | | | | | | |
|---|---|---|---|---|---|---|---|
| **Year** | **2015** | **2016** | **2017** | **2018** | **2019** | **2020** | ***Diff 2015/2020 (%)*** |
| TSMC | 1 566 662 | 1 648 268 | 1 638 051 | 1 705 746 | 1 678 753 | 2 150 339 | *37* |
| Innolux | 428 000 | 440 000 | 425 000 | 365 000 | 348 000 | 323 000 | *-25* |
| Unimicron | 15 342 | 16 350 | 16 026 | 18 546 | 17 835 | 20 047 | *31* |
| UMC | 621 400 | 616 000 | 603 958 | 595 576 | 512 741 | 539 321 | *-13* |
| Powerchip | 46 466 | 59 604 | 89 378 | 107 183 | 95 781 | 107 931 | *132* |
| Vanguard | 192 600 | 272 000 | 273 100 | 331 100 | 286 800 | 236 600 | *23* |
| Global Wafers | 225 | 1 160 | 1 737 | 1 834 | 1 503 | 1 570 | *598* |
| Nanya | 51 261 | 51 584 | 59 751 | 78 311 | 88 700 | 90 327 | *76* |
| Winbond | 51 725 | 63 673 | 62 318 | 64 510 | 65 749 | 53 271 | *3* |
| Epistar | 21 237 | 21 569 | 31 648 | 23 530 | 16 519 | 38 444 | *81* |
| Win Semiconductors | 41 637 | 48 743 | 54 516 | 64 447 | 66 342 | 76 890 | *85* |
| Nuvoton | 32 000 | 34 400 | 39 100 | 35 800 | 311 000 | 362 000 | *1031* |
| Lextar | 44 884 | 44 354 | 40 663 | 51 815 | 41 909 | 52 998 | *18* |
| Everlight | ND* | ND* | ND* | 903 | 979 | 912 | |
| Optotech | ND* | ND* | ND* | ND* | ND* | ND* | |
| Wafer Works | 5 433 | 7 729 | 9 807 | 10 778 | 11 455 | 6 506 | *20* |
| **Subtotal** | **3 120 887** | **3 327 450** | **3 347 070** | **3 457 097** | **3 546 085** | **4 062 176** | *30* |
| All ECM except TSMC | | | | | | | |

| | Greenhouse Gases Emissions (Scope 2) | | | | | | |
|---|---|---|---|---|---|---|---|
| **Year** | **2015** | **2016** | **2017** | **2018** | **2019** | **2020** | ***Diff 2015/2020 (%)*** |
| TSMC | 4 315 766 | 5 030 647 | 5 702 511 | 6 325 931 | 6 673 235 | 7 429 951 | *72* |
| Innolux | 2 388 000 | 2 277 000 | 2 690 000 | 2 878 000 | 2 778 000 | 3 059 000 | *28* |
| Unimicron | 406 583 | 414 532 | 434 028 | 520 861 | 519 528 | 520 922 | *28* |
| UMC | 1 167 200 | 1 186 000 | 1 356 000 | 1 365 000 | 1 318 000 | 1 287 248 | *10* |
| Powerchip | 424 788 | 436 077 | 569 192 | 552 566 | 548 034 | 565 108 | *33* |
| Vanguard | 435 000 | 449 100 | 438 000 | 456 500 | 440 700 | 434 600 | *0* |
| Global Wafers | 10 765 | 151 208 | 155 148 | 200 281 | 173 491 | 167 357 | *1455* |
| Nanya | 218 972 | 238 436 | 316 442 | 369 904 | 390 021 | 379 417 | *73* |
| Winbond | 200 861 | 206 302 | 250 859 | 265 596 | 268 947 | 278 046 | *38* |
| Epistar | 138 577 | 166 322 | 159 869 | 165 396 | 152 820 | 192 007 | *39* |
| Win Semiconductors | 71 281 | 82 874 | 96 562 | 101 253 | 104 151 | 114 953 | *61* |
| Nuvoton | 41 000 | 40 800 | 41 600 | 39 400 | 38 900 | 36 800 | *-10* |
| Lextar | 52 818 | 50 895 | 48 418 | 49 031 | 39 244 | 36 323 | *-31* |
| Everlight | ND* | ND* | ND* | 111 716 | 102 699 | 103 020 | |
| Optotech | ND* | ND* | ND* | ND* | ND* | ND* | |
| Wafer Works | 55 593 | 60 840 | 67 405 | 68 642 | 64 459 | 62 035 | *12* |
| **Subtotal** | **9 929 219** | **10 793 049** | **12 328 051** | **13 472 095** | **13 614 248** | **14 668 807** | *48* |

| | Greenhouse Gases Emissions (Scope 3) | | | | | | |
|---|---|---|---|---|---|---|---|
| **Year** | 2015 | 2016 | 2017 | 2018 | 2019 | 2020 | *Diff 2015/2020 (%)* |
| TSMC | 3 446 138 | 3 770 912 | 4 242 521 | 4 315 497 | 5 307 028 | 5 511 486 | *60* |
| Innolux | 18 000 | 25 000 | 22 000 | 14 000 | 10 000 | 28 000 | *56* |
| Unimicron | 423 | 320 | 731 | 837 | 880 | 320 205 | *75599* |
| UMC | 2 514 200 | 3 642 000 | 2 218 000 | 1 968 000 | 2 073 000 | 2 260 902 | *-10* |
| Powerchip | ND | ND | ND | ND | ND | ND | |
| Vanguard | ND | ND | 214 001 | 235 512 | ND | ND | |
| Global Wafers | ND | ND | ND | ND | ND | ND | |
| Nanya | ND | ND | ND | ND | 902 293 | 1 073 295 | |
| Winbond | ND | ND | ND | ND | ND | ND | |
| Epistar | ND | ND | ND | ND | ND | ND | |
| Win Semiconductors | ND | ND | ND | ND | ND | ND | |
| Nuvoton | ND | ND | ND | ND | ND | ND | |
| Lextar | ND | ND | ND | ND | ND | ND | |
| Everlight | ND | ND | ND | ND | ND | ND | |
| Optotech | ND | ND | ND | ND | ND | ND | |
| Wafer Works | ND | 113 285 | 114 731 | 138 760 | 197 381 | 1 667 346 | |
| **Subtotal** | | | | | | | |
| | | | | | | | All ECM except TSM |

| | Total Greenhouse Gases Emissions (Scope 1+2) | | | | | | | | |
|---|---|---|---|---|---|---|---|---|---|
| **Year** | **2015** | **2016** | **2017** | **2018** | **2019** | **2020** | **Diff 2015/2020 (%)** | ***Notes*** | ***Sources*** |
| TSMC | 5 882 428 | 6 678 915 | 7 340 562 | 8 031 677 | 8 351 988 | 9 580 290 | *63* | *0.554 kg of CO2e / kWh* | *TSMC CSR Report 2019-2021* |
| Innolux | 2 816 000 | 2 717 000 | 3 115 000 | 3 243 000 | 3 126 000 | 3 382 000 | *20* | | *Innolux CSR Report 2019-2020* |
| Unimicron | 421 925 | 430 882 | 450 054 | 539 407 | 537 363 | 540 969 | *28* | | *Unimicron CSR Report 2019-2020* |
| UMC | 1 788 600 | 1 802 000 | 1 959 958 | 1 960 576 | 1 830 741 | 1 826 569 | *2* | *0.533 kg of CO2e / kWh* | *UMC CSR Report 2019-2020* |
| Powerchip | 471 254 | 495 681 | 658 570 | 659 749 | 643 815 | 673 039 | *43* | | *Powerchip CSR Report 2019-2020* |
| Vanguard | 627 600 | 721 100 | 711 100 | 787 600 | 727 500 | 671 200 | *7* | *New FabVS1 in Singapore is not counted* | *Vanguard CSR Report 2019-2020* |
| Global Wafers | 10 990 | 152 368 | 156 885 | 202 115 | 174 994 | 168 927 | *1437* | | *GlobalWafers CSR Report 2019-2020* |
| Nanya | 270 233 | 290 020 | 376 193 | 448 215 | 478 721 | 469 744 | *74* | | *Nanya CSR Report 2015-2016-2019-2020* |
| Winbond | 252 586 | 269 975 | 313 177 | 330 106 | 334 696 | 331 317 | *31* | | *Winbond CSR Report 2017-2018-2020* |
| Epistar | 159 814 | 187 891 | 191 517 | 188 926 | 169 339 | 230 451 | *44* | *Might include 1 small Chinese facility* | *Epistar CSR Report 2018-2020* |
| Win Semiconductors | 112 918 | 131 617 | 151 078 | 165 700 | 170 493 | 191 843 | *70* | | *Win CSR Report 2018-2019-2020* |
| Nuvoton | 73 000 | 75 200 | 80 700 | 75 200 | 349 900 | 398 800 | *446* | | *Nuvoton CSR Report 2019-2020* |
| Lextar | 97 702 | 95 249 | 89 081 | 100 846 | 81 153 | 89 321 | *-9* | | *Lextar CSR Report 2016-2017-2018-2020* |
| Everlight | ND* | ND* | ND* | 112 619 | 103 678 | 103 932 | | | *Everlight CSR Report 2019* |
| Optotech | 37 127 | 39 782 | 39 419 | 42 135 | 41 945 | 41 945 | *13* | *Scopes not detailed* | *Optotech CSR Report 2017-2019* |
| Wafer Works | 61 026 | 68 568 | 77 212 | 79 420 | 75 914 | 68 541 | *12* | *Location-based data, might include 1 smal* | *Wafer Works CSR Report 2016-2018-2020* |
| **Subtotal** | **13 085 218** | **14 158 264** | **15 712 523** | **16 969 309** | **17 200 259** | **18 770 908** | *43* | | |
| All ECM except TSMC | 7 202 790 | 7 479 349 | 8 371 961 | 8 937 632 | 8 848 271 | 9 190 618 | | | |

ND = No Data

(*) : CSR department contacted but didn't answer

## Greenhouse Gases emissions (GHG) in Taiwan

| ***Unit : metric tons CO2e*** | | | | | | | | |
|---|---|---|---|---|---|---|---|---|
| **Year** | **2015** | **2016** | **2017** | **2018** | **2019** | **2020** | ***Diff 2015/2020 (%)*** | **Source** |
| National GHG Emissions | 260 200 000 | 264 740 000 | 271 220 000 | 268 850 000 | 260 400 000 | | | MOEA, Energy Statistics Handbook 2020 (p. 126) ; https://eng.stat.gov.tw/ct.asp?xItem=18741&CtNode=4942&mp=5 ; Data for IC/semiconductor industry (p. 76) https://unfccc.saveoursky.org.tw/nir/2021nir/uploads/04_content.pdf + https://unfccc.saveoursky.org.tw/nir/tw_nir_2021.php ; (2020 |
| Industry GHG emissions | 126 330 000 | 127 590 000 | 131 210 000 | 132 950 000 | 127 070 000 | | | |
| IC and semiconductor industry GHG emissions | 31 720 000 | 30 720 000 | 30 220 000 | 33 370 000 | 32 670 000 | | | |
| Industry share of national GHG emissions | 48,6 | 48,2 | 48,4 | 49,5 | 48,8 | | | |
| **Study perimeter** | | | | | | | | |
| **THIS STUDY – Scope 1+2 Emissions of selected ECM** | **13 085 218** | **14 158 264** | **15 712 523** | **16 969 309** | **17 200 259** | **18 770 908** | *43,5* | |
| Share of Industry GHG emissions | 10,4 | 11,1 | 12,0 | 12,8 | 13,5 | | | |
| Share of National GHG emissions | 5,0 | 5,3 | 5,8 | 6,3 | 6,6 | | | |
| **Other sectors** | | | | | | | | |
| Agriculture GHG emissions | 2 830 000 | 2 830 000 | 2 890 000 | 3 100 000 | 3 070 000 | | | |
| Transport GHG emissions | 37 040 000 | 38 150 000 | 37 830 000 | 36 790 000 | 37 000 000 | | | |
| Services GHG emissions | 28 710 000 | 29 160 000 | 30 550 000 | 28 440 000 | 27 140 000 | | | |
| Residential GHG emissions | 28 050 000 | 29 640 000 | 30 780 000 | 29 460 000 | 28 500 000 | | | |
| Industry GHG emissions | 126 330 000 | 127 590 000 | 131 210 000 | 132 950 000 | 127 070 000 | | | |
| Energy GHG emissions | 37 240 000 | 37 380 000 | 37 960 000 | 38 120 000 | 37 630 000 | | | |

## Greenhouse Gases emissions (GHG) in Taiwan

| ***Unit : %*** | | | | | | | | | |
|---|---|---|---|---|---|---|---|---|---|
| **Year** | **2015** | **2016** | **2017** | **2018** | **2019** | **2020** | *(min)* | *(max)* | *(average)* |
| Share of scope 2 with respect to total (scope 1+2) | 75,9 | 76,2 | 78,5 | 79,4 | 79,2 | 78,1 | *75,9* | *79,4* | *77,9* |

# Water consumption of selected electronic components manufacturers

| *Unit : m3* | Water consumption | | | | | | | |
|---|---|---|---|---|---|---|---|---|
| **Year** | **2015** | **2016** | **2017** | **2018** | **2019** | **2020** | ***Diff 2015/2020 (%)*** | **Source** |
| TSMC | 34 000 000 | 38 600 000 | 45 200 000 | 51 000 000 | 58 000 000 | 70 600 000 | *108* | TSMC CSR Report 2019-2021 |
| Innolux | 24 190 000 | 22 950 000 | 25 040 000 | 21 830 000 | 20 210 000 | 20 415 000 | *-16* | Innolux CSR Report 2019-2020 |
| Unimicron | 18 752 000 | 13 061 106 | 13 140 492 | 14 614 868 | 15 306 000 | 15 007 898 | *-20* | Unimicron CSR Report 2019-2020 |
| UMC | 13 830 000 | 14 456 000 | 14 900 000 | 14 910 000 | 14 810 000 | 15 500 000 | *12* | UMC CSR Report 2019-2020 |
| Powerchip | 3 678 669 | ND* | ND* | 1 451 979 | 1 497 624 | 1 560 296 | | Powerchip CSR Report 2019-2020 |
| Vanguard | 4 540 000 | 4 780 000 | 4 860 000 | 4 990 000 | 4 980 000 | 6 560 000 | *44* | Vanguard CSR Report 2019-2020 |
| Global Wafers | 545 097 | 3 639 324 | 3 664 318 | 5 469 000 | 4 960 000 | 4 324 000 | *693* | GlobalWafers CSR Report 2019-2020 |
| Nanya | 2 198 960 | 2 244 759 | 3 092 814 | 3 022 362 | 3 258 386 | 3 368 954 | *53* | Nanya CSR Report 2015-2016-2019-2020 |
| Winbond | 2 320 000 | 2 340 000 | 2 830 000 | 945 000 | 979 000 | 1 216 000 | *-48* | Winbond CSR Report 2017-2018-2020 |
| Epistar | ND* | 450 000 | 420 000 | 410 000 | 380 000 | 370 000 | | Epistar CSR Report 2018-2020 |
| Win Semiconductors | ND* | ND* | 253 101 | 214 044 | 208 239 | 255 063 | | Win CSR Report 2018-2019-2020 |
| Nuvoton | 387 000 | 420 000 | 442 000 | 440 000 | 395 000 | 401 000 | *4* | Nuvoton CSR Report 2019-2020 |
| Lextar | ND* | ND* | ND* | 98 470 | 83 750 | 76 410 | | Lextar CSR Report 2016-2017-2018-2020 |
| Everlight | ND* | ND* | ND* | 994 490 | 874 770 | 849 600 | | Everlight CSR Report 2019-2020 |
| Optotech | 1 194 967 | 1 272 536 | 1 336 185 | 1 422 818 | 1 402 261 | 1 402 261 | *17* | Optotech CSR Report 2017-2019 |
| Wafer Works | 1 570 607 | 1 713 684 | 1 836 680 | 2 166 502 | 2 166 502 | 2 133 853 | *36* | Wafer Works CSR Report 2016-2018-2020 |
| **Subtotal** | **107 207 300** | **105 927 409** | **117 015 590** | **123 979 533** | **129 511 532** | **144 040 335** | *34* | |
| All ECM except TSMC | 73 207 300 | 67 327 409 | 71 815 590 | 72 979 533 | 71 511 532 | 73 440 335 | | |

ND = No Data

(*) : CSR department contacted but didn't answer

CSR reports are sometimes unclear about their reporting, it is difficult to understand if they're reporting water intake, water consumption including recycled water or their net water consumption. The numbers presented here should rather viewed as water intake or water footprint.

# Domestic water consumption in Taiwan

| *Unit : m3* | Water consumption | | | | | | | |
|---|---|---|---|---|---|---|---|---|
| **Year** | **2015** | **2016** | **2017** | **2018** | **2019** | **2020** | **Diff 2015/2020 (%)** | **Source** |
| National water consumption | 16 025 000 000 | 16 546 000 000 | 16 645 000 000 | 16 713 000 000 | 16 739 280 000 | 16 675 930 000 | *4* | Utilization of Water Resources (2016-2019) https://www.wra.gov.tw/News.aspx?n=2953&sms=9084&_CSN=0 ; https://www.wra.gov.tw/News_Content.aspx?n=2945&s=7394 |
| Industry water consumption | 1 601 000 000 | 1 629 000 000 | 1 654 000 000 | 1 668 000 000 | 1 671 350 000 | 1 803 190 000 | *13* | |
| Industry share of national consumption | 10,0 | 9,8 | 9,9 | 10,0 | 10,0 | 10,8 | | |
| **Study perimeter** | | | | | | | | |
| **THIS STUDY – Water consumption of s** | **107 207 300** | **105 927 409** | **117 015 590** | **123 979 533** | **129 511 532** | **144 040 335** | ***34,4*** | |
| Share of Industry water consumption | 6,7 | 6,5 | 7,1 | 7,4 | 7,7 | 8,0 | | |
| Share of National water consumption | 0,7 | 0,6 | 0,7 | 0,7 | 0,8 | 0,9 | | |
| **Other sectors** | | | | | | | | |
| Agriculture water consumption | 10 497 740 000 | 11 086 030 000 | 11 200 240 000 | 11 890 000 000 | 11 363 500 000 | 11 592 470 000 | *10* | |
| Industry water consumption | 1 601 000 000 | 1 629 000 000 | 1 654 000 000 | 1 668 000 000 | 1 671 350 000 | 1 803 190 000 | *13* | |
| Domestic water consumption (household | 3 142 230 000 | 3 183 410 000 | 3 147 140 000 | 3 155 810 000 | 3 185 510 000 | 3 280 270 000 | *4* | |

# Indexes of Industrial Production in Taiwan

***2016=100***

| Year | 2015 | 2016 | 2017 | 2018 | 2019 | 2020 | Notes | Sources |
|---|---|---|---|---|---|---|---|---|
| **Manufacture of Integrated Circuits** | 88,1 | 100,0 | 109,4 | 119,0 | 120,7 | 153,9 | *SCOPE* | MOEA |
| Manufacture of Discrete Devices | 96,0 | 100,0 | 109,3 | 128,3 | 124,3 | 130,0 | *SCOPE* | |
| Packaging and Testing of Semi-conductors | 99,8 | 100,0 | 103,8 | 108,3 | 116,6 | 123,8 | *OUT OF SCOPE* | |
| Manufacture of Electronic Passive Devices | 94,9 | 100,0 | 109,4 | 151,0 | 104,9 | 120,7 | *SCOPE* | |
| Manufacture of Bare Printed Circuit Boards | 99,6 | 100,0 | 108,7 | 109,7 | 107,4 | 120,1 | *OUT OF SCOPE* | |
| Manufacture of Liquid Crystal Panel and Components | 110,7 | 100,0 | 117,7 | 113,5 | 102,5 | 108,4 | *OUT OF SCOPE* | |
| Manufacture of Light Emitting Diodes (LED) | 118,6 | 100,0 | 91,2 | 84,0 | 69,0 | 64,5 | *SCOPE* | |
| Manufacture of Solar Cells | 110,1 | 100,0 | 83,4 | 74,0 | 46,2 | 44,5 | *OUT OF SCOPE* | |
| Manufacture of Other Optoelectronic Materials and Components | 105,8 | 100,0 | 88,8 | 84,5 | 83,3 | 82,5 | *SCOPE* | |
| Manufacture of Printed Circuit Assembly | 95,2 | 100,0 | 101,2 | 102,9 | 138,0 | 193,9 | *OUT OF SCOPE* | |
| Manufacture of Other Electronic Parts and Components (Not Elsewhere Classified) | 99,2 | 100,0 | 89,9 | 90,1 | 122,6 | 153,7 | *SCOPE* | |
| Manufacture of Electronic Parts and Components (overall) | **95,6** | **100,0** | **108,2** | **114,0** | **114,1** | **136,3** | | |

# Taiwan emissions reduction roadmap

| *Unit: Megaton CO2e* | 2005 | 2006 | 2007 | 2008 | 2009 | 2010 | 2011 | 2012 | 2013 | 2014 | 2015 | 2016 | 2017 | 2018 | 2019 | 2020 |
|---|---|---|---|---|---|---|---|---|---|---|---|---|---|---|---|---|
| National GHG emissions | 249,72 | 257,12 | 261,00 | 249,24 | 237,53 | 253,43 | 258,84 | 254,90 | 255,78 | 260,20 | 260,20 | 264,74 | 271,22 | 268,85 | 260,40 | ND |
| Data from Chou (FIG. 5) - Energy Bureau 2018 | 17,6545 | 17,4953 | 18,7724 | 19,5274 | 18,2665 | 20,5241 | 21,724 | 22,1293 | 22,9983 | 23,7802 | 24,614 | 25,6552 | | | | |
| Targets | | | | | | | | | | | | | | | | 244,7 |
| THIS STUDY – Sample's GHG Emissions (Sc1+2) | | | | | | | | | | | 13,09 | 14,16 | 15,71 | 16,97 | 17,20 | 18,77 |
| THIS STUDY – Scenario 1 | | | | | | | | | | | | | | | | 18,77 |
| THIS STUDY – Scenario 2 | | | | | | | | | | | | | | | | 18,77 |
| THIS STUDY – Scenario 3 | | | | | | | | | | | | | | | | 18,77 |
| THIS STUDY – Sub-sector's GHG Emissions (Sc1+2) | | | | | | | | | | | 20,99 | 22,71 | 23,87 | 24,16 | 30,55 | 32,40 |

| *Unit: Megaton CO2e* | *2021* | 2022 | *2023* | 2024 | *2025* | 2026 | *2027* | 2028 | *2029* | 2030 | *2031* | 2032 | *2033* | 2034 | *2035* |
|---|---|---|---|---|---|---|---|---|---|---|---|---|---|---|---|
| National GHG emissions | | | | | | | | | | | | | | | |
| Data from Chou (FIG. 5) - Energy Bureau 2018 | | | | | | | | | | | | | | | |
| Targets | | | | | 224,7 | | | | | 199,8 | | | | | |
| THIS STUDY – Sample's GHG Emissions (Sc1+2) | | | | | | | | | | | | | | | |
| THIS STUDY – Scenario 1 | *20,18* | *21,69* | *23,31* | *25,05* | *26,93* | *28,94* | *31,11* | *33,44* | *35,94* | *38,63* | *41,52* | *44,62* | *47,96* | *51,55* | *55,41* |
| THIS STUDY – Scenario 2 | *19,34* | *19,92* | *20,52* | *21,14* | *21,77* | *22,43* | *23,10* | *23,80* | *24,52* | *25,26* | *26,02* | *26,80* | *27,61* | *28,44* | *29,30* |
| THIS STUDY – Scenario 3 | *18,77* | *18,77* | *18,77* | *18,77* | *18,77* | *18,77* | *18,77* | *18,77* | *18,77* | *18,77* | *18,77* | *18,77* | *18,77* | *18,77* | *18,77* |
| THIS STUDY – Sub-sector's GHG Emissions (Sc1+2) | | | | | | | | | | | | | | | |

| *Unit: Megaton CO2e* | 2036 | *2037* | 2038 | *2039* | 2040 | *2041* | 2042 | *2043* | 2044 | *2045* | 2046 | *2047* | 2048 | *2049* | 2050 |
|---|---|---|---|---|---|---|---|---|---|---|---|---|---|---|---|
| National GHG emissions | | | | | | | | | | | | | | | |
| Data from Chou (FIG. 5) - Energy Bureau 2018 | | | | | | | | | | | | | | | |
| Targets | | | | | | | | | | | | | | | 124,9 |
| THIS STUDY – Sample's GHG Emissions (Sc1+2) | | | | | | | | | | | | | | | |
| THIS STUDY – Scenario 1 | *59,56* | *64,01* | *68,81* | *73,95* | *79,49* | *85,44* | *91,83* | *98,70* | *106,09* | *114,03* | *122,56* | *131,73* | *141,59* | *152,18* | *163,57* |
| THIS STUDY – Scenario 2 | *30,18* | *31,10* | *32,03* | *33,00* | *34,00* | *35,03* | *36,08* | *37,17* | *38,30* | *39,46* | *40,65* | *41,88* | *43,14* | *44,45* | *45,79* |
| THIS STUDY – Scenario 3 | *18,77* | *18,77* | *18,77* | *18,77* | *18,77* | *18,77* | *18,77* | *18,77* | *18,77* | *18,77* | *18,77* | *18,77* | *18,77* | *18,77* | *18,77* |
| THIS STUDY – Sub-sector's GHG Emissions (Sc1+2) | | | | | | | | | | | | | | | |

**GHG Reduction Targets (base year 2005)**

| | Year | Relative (w.r.t. 2005) | Absolute target |
|---|---|---|---|
| 1st phase (2016-2020) | 2020 | -2% | 244,7 |
| 2nd phase (2021-2025) | 2025 | -10% | 224,7 |
| 3rd phase (2026-2030) | 2030 | -20% | 199,8 |
| Final objective (2030-2050) | 2050 | -50% | 124,9 |

*Notes*

Greenhouse Gas Reduction and Management Act (溫室氣體減量及管理法) Preannounced to Change Name to Climate Change Response Act. The national long-term reduction goal is to, by 2050, lower carbon emissions to 50% of the amount emitted in 2005

*Sources*

https://www.epa.gov.tw/eng/F7AB26007B8FE8DF/74023638-a2ee-4d1f-ad5a-8941a2415ba2 ; https://ghgrule.epa.gov.tw/eng_article/index/15 ; https://apps.fas.usda.gov/newgainapi/api/Report/DownloadReportByFileName?fileName=Taiwan%20Climate%20Change%20Overview_Taipei_Taiwan_11-29-2021.pdf

**Prospective scenarios**

| | Year | CAGR improvement carbon intensity | CAGR increase manufacturing | Resulting CAGR |
|---|---|---|---|---|
| Scenario 1 : BAU (Maintaned growth in manufacturing (unrealistic)) | 2020-2050 | 0,000 | 0,075 | **0,075** |
| Scenario 2 : Manufacturing & Efficiency (Best effort for intensity while inc | 2020-2050 | -0,006 | 0,035 | **0,029** |
| Scenario 3 : Constant (Stabilization to 2020 value, whatever intensity an | 2020-2050 | 0,000 | 0,000 | **0,000** |

from Chou and Energy Bureau : The planning for the reduction pathway would also rely on the technological breakthroughs and supporting measures to allow energy intensity and electricity generation to improve by 2.4% and 2%, respectively, from 2017 to 2025

| | |
|---|---|
| This yields a CAGR of : | -0,006 |
| if based on EU-27 improvements (fig 13) : https://www.sciencedirect.com | -0,024 |
| Chou et al. CAGR for electronics GHG emissions | 3,46% |
| CAGR of National GHG emissions (2005-2019) | 0,30% |
